# Supplementary material for: Dark Solitons in Waveguide Polariton Fluids Shed Light on Interaction Constants
Source: arXiv:1703.08351 ancillary file (2017-03-24)
Supplement: Supplementary file 1 [file Supplementary_Information.pdf]

# Supplementary Information On : Dark Solitons in Waveguide Polariton Fluids Shed Light on Interaction Constants

P. M. Walker,[1,*] L. Tinkler,[1] B. Royall,[1] D. V. Skryabin,[2,3] I. Farrer,[4] D. A. Ritchie,[5] M. S. Skolnick,[1] and D. N. Krizhanovskii[1]

[1]*Department of Physics and Astronomy, University of Sheffield, S3 7RH Sheffield, UK*
[2]*Department of Physics, University of Bath, BA2 7AY Bath, UK*
[3]*ITMO University, Kronverksky Avenue 49, St. Petersburg 197101, Russia*
[4]*Department of Electronic and Electrical Engineering, University of Sheffield, S3 7HQ Sheffield, UK*
[5]*Cavendish Laboratory, University of Cambridge, CB3 0HE Cambridge, UK*

## S1. Experimental Arrangement

The sample used in this work is a planar semiconductor waveguide grown by molecular beam epitaxy (MBE), similar to that used is Ref. 3. The GaAs core of total thickness 135nm contains three 10nm wide $In_{0.04}Ga_{0.96}As$ quantum wells separated by 10nm GaAs barriers. On one side the core is separated from the GaAs substrate by a 500nm $Al_{0.9}Ga_{0.1}As$ cladding layer while on the other it is separated from air by a 200nm PECVD-grown silicon nitride cladding layer. The sample was mounted in a continuous flow liquid helium cryostat and held at 10 Kelvin. A schematic of the experimental arrangement is shown in Fig. 1(a) in the main text. A continuous wave (CW) multi-mode Ti:Sapphire laser tuned to an energy $\delta = -3.8$meV below the exciton resonance was directed onto the sample surface using a microscope objective. The incident light was coupled into the structure using a diffractive grating coupler with period 250 nm. The angle of incidence, wavelength and polarisation of the laser beam were chosen to match those of the waveguide transverse electric (TE) guided mode. Along with the position of the laser spot relative the input grating coupler they were tuned to maximise the power observed at the output grating coupler. Coupled light propagated a distance $L = 600$ µm in the waveguide and was coupled out through another grating after which it was collected by the same objective and imaged onto a CCD camera. The phase of the output field was measured by interfering the output light on the CCD with a flat-phase Gaussian reference beam derived from the input laser. The incident laser power was varied over four orders of magnitude between 2 µW and 33 mW.

We study initial conditions containing both phase and intensity jumps. The phase jump initial condition was generated by expanding the laser beam to approximately 3mm diameter and passing it through a phase mask manufactured by reactive ion etching of a glass cover-slip to remove material corresponding to half a wavelength of light. Since the light passing through one half of the plate travels further there is a phase jump across the beam centered on the interface between etched and unetched regions. The modified laser spot was imaged onto the input grating on the sample surface with a demagnification of 100 times. In the case of the amplitude discontinuity the laser was expanded, passed across a metal wire to remove some intensity from the beam, and imaged back onto the sample.

## S2. Coupling Efficiency

The power coupled to the guided mode was measured in the following way. The laser power before the objective, beamsplitter, mirrors and cryostat windows was measured with a commercial power meter. Using the same meter it was determined that the power at the sample surface was 0.19 ± 0.01 times smaller than at the previous position. The power coming from the output grating was also measured by placing the meter after a spatial filter centered on the output grating. The ratio of the power at the spatial filter is again 0.19±0.01 times the power directly after the grating coupler due to losses at the beamsplitter, objective, windows and lenses. The power incident on the input grating versus that immediately after the output grating is plotted in Fig. S1(a-c) for a few detunings of the polariton energy relative to the exciton. Fitting the linear region at low powers gives the ratio between the two, which is given by the expression $P_{\mathrm{out}} = P_{\mathrm{inc}} \cdot (\kappa_{\mathrm{up}}/\kappa)^2 \cdot F \cdot \exp(-L/L_{\mathrm{loss}})$. Here $\kappa_{\mathrm{up}}$ is the coupling rate between the guided mode and free space modes in the direction away from the substrate, e.g. the direction from which the laser is coupled and the output light is collected[49]. The value $\kappa$ is the coupling rate of the guided mode to all modes including substrate photonic modes and absorption in the coupler region. The exponential contains the losses in the region between the couplers while $F$ is the $z$-direction overlap integral between the exponential mode profile of the grating and the gaussian mode profile of the excitation spot[49]. This overlap integral varies very slowly with spot size and since the coupling was optimised experimentally on each run the value will be very close to the theoretical maximum of 0.8. The losses in between the gratings were measured as in Ref. 3 and are shown in Fig. S1(d). Taking all these measured quantities into account we are able to deduce $\kappa_{\mathrm{up}}/\kappa$ and hence the input coupling efficiency given by[49] $\eta = (\kappa_{\mathrm{up}}/\kappa)F$. We plot the coupling efficiency as a function of detuning in Fig. S1(e). We note that the output coupling efficiency, in the sense of the fraction of power leaving the sample in the direction towards the micro-

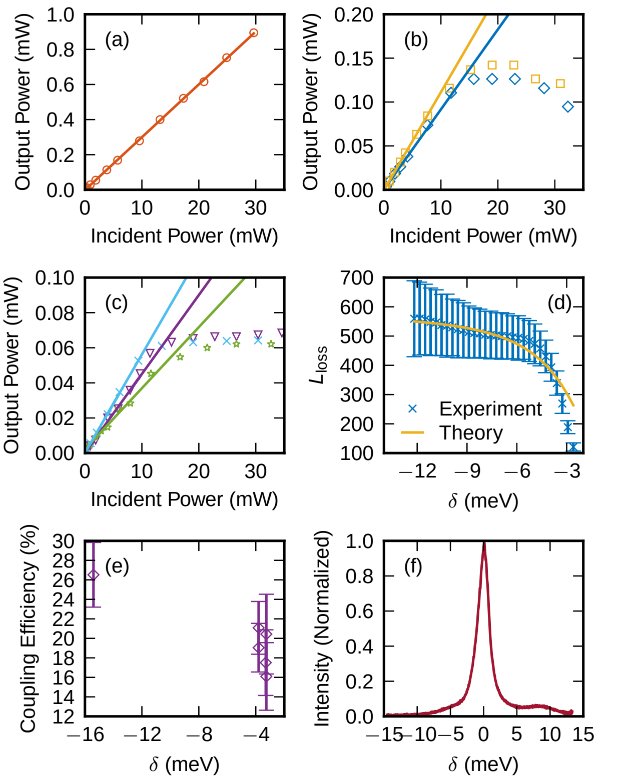


FIG. S1. Power output from waveguide vs. coupled input power for detunings (a)$\hbar\delta$=-15.4meV, (b)$\hbar\delta$=-3.8meV, (c)$\hbar\delta$=-3.3meV. Different lines on the same panel correspond to different transverse profiles. (d) Experimental (points) and model (solid line) polariton loss length vs. detuning. (e) Coupling efficiency vs. detuning. (f) Photoluminescence spectrum of exciton line in the grating coupler region.

scope objective, is given by $\kappa_{up}/\kappa$. At a detuning of -15.4meV where the system is effectively purely photonic we obtain $\eta$ =27±3%. The ratio of upward to total coupling rates in the purely photonic case was independently determined by modelling the structure using the FDTD method. From this we obtained $\kappa_{up}/\kappa = 1/3$. The expected incoupling efficiency is then $\eta$ =0.8/3=26.6%, in very good agreement with the experimental measurement for the strongly photonic case. Combining the two results at the detuning of -3.8meV used in this paper we deduce $\eta$=20±2%, which is slightly less than the purely photonic case. The values at 3.3meV are even less. We therefore attribute the slight reduction in coupling efficiency to the absorption of a fraction of the light at the injection site in the tail of the inhomogeneously broadened exciton line. This is supported by the photoluminescence spectrum in Fig. S1(f) taken in the grating region near zero angle where there are no polaritons. It can be seen that the tail extends over the detunings of -3.8meV and -3.3meV.

## S3. Evolution Equations

Polaritons propagating in the waveguide are in general desribed by coupled equations (1) for the photon and exciton fields and, in our case, an additional incoherent exciton reservoir. The parameters are defined in the main text and also, in more detail, below.

$$\left(i\frac{\partial}{\partial t} + i\gamma_{\rm p} + v_{\rm g}\left(i\frac{\partial}{\partial z} + \frac{1}{2\beta_{\rm e}}\frac{\partial^2}{\partial x^2}\right)\right)A = \left(\frac{\Omega}{2}\right)\psi \quad (1a)$$

$$\left(i\frac{\partial}{\partial t} + i\left(\gamma_{\rm e} + \gamma_{\rm r}\right) - g_{\rm X}\left(|\psi|^2 + n_{\rm R}\right)\right)\psi = \left(\frac{\Omega}{2}\right)A \quad (1b)$$

$$\frac{\partial n_{\rm R}}{\partial t} = 2\gamma_{\rm r}|\psi|^2 - 2\gamma_{\rm R}n_{\rm R} \quad (1c)$$

In this description the optical electric field is fixed in the transverse electric (TE) linear polarisation (along the x-axis) since the TM polarised guided mode is spectrally separated, very lossy due to being close to cutoff and incorrectly polarised to couple strongly to the in-plane exciton dipoles. The photon field and exciton polarisation field are described by $E = A(x,t,z)\exp(i\beta_{\rm e}z - i\omega_{\rm e}t)$ and $\Psi = \psi(x,t,z)\exp(i\beta_{\rm e}z - i\omega_{\rm e}t)$ where $A$ and $\psi$ are the photon and exciton amplitudes which vary slowly compared to the exciton frequency $\omega_{\rm e}$ and the waveguide propagation constant (wavenumber) at the exciton frequency $\beta_{\rm e}$. In obtaining Eqn. (1a) we have used the paraxial or slowly-varying-envelope approximation which proceeds as follows. The spatial part of the standard electromagnetic wave equation contains the term $\partial^2 E/\partial z^2$. We expand this as $\left(\partial^2 A/\partial z^2 + 2i\beta_{\rm e}\partial A/\partial z + \beta_{\rm e}^2\right)\exp(i\beta_{\rm e}z - i\omega_{\rm e}t)$ and note that since $A(z)$ varies on a length scale very long compared to the wavelength $2\pi/\beta_{\rm e}$ we can discard the highest order dervative $\partial^2 A/\partial z^2$. This approximation is a good one in a waveguide system such as ours because the wavenumber is large. The effect of the waveguide confinement in the $y$-direction is, in general, to introduce dispersive terms $\beta_m\partial^m A/\partial t^m$, where $m$ is an integer, into the photon field equation (1a)[4]. We neglect the photonic dispersion for $m > 1$ because its contribution to the polariton dispersion is negligible in comparison to that arising from the light-matter coupling[2]. The photon dispersion relation is then approximated as a linear function $\omega_{\rm ph} = \omega_{\rm e} + v_{\rm g}(\beta - \beta_{\rm e})$ where $v_{\rm g}$ is the photonic group velocity. We obtained the dispersive parameters of the system experimentally by fitting the angle-resolved photoluminescence spectrum (see Fig.1(b) in the main text and Ref. 3 for more details). We find $\omega_{\rm e}$ =2253 ps$^{-1}$, $\beta_{\rm e} = 23.65\mu{\rm m}^{-1}$ and $v_{\rm g}$ =58μm ps$^{-1}$. The other quantities in Eqns. (1) are defined as follows. The photon losses are $\gamma_{\rm p}$ and the loss term $\gamma_{\rm r}$ in the exciton field represents scattering of excitons to an incoherent reservoir containing number density $n_{\rm R}$ described by Eqn. (1c). All other contributions to the linewidth of the strongly-coupled excitons are described by $\gamma_{\rm e}$. The loss from the incoherent

reservoir is given by $\gamma_R$. The nonlinear interaction is provided by renormalization of the strongly-coupled exciton field proportional to the total density of strongly-coupled and reservoir excitons, with strength given by the constant $g_X$.

We search for steady state solutions $\partial n_R/\partial t = 0$, so that Eqn. (1c) gives $n_R = (\gamma_r/\gamma_R)\,|\psi|^2$. The physical meaning of this model is that scattering from the coherent excitonic part of the polaritons populates an incoherent reservoir. At long times the population of this reservoir stabilises at a value where the loss rate balances the excitons entering from the coherent state. Substituting this reservoir population expression into Eqn. (1b) the nonlinearity $g_X(|\psi|^2 + n_R)$ becomes $g_{\rm eff}\,|\psi|^2$ where $g_{\rm eff} = g_X\,(1 + \gamma_r/\gamma_R)$ is an effective exciton-exciton scattering which accounts for the fact that for every coherent exciton the reservoir contains another $\gamma_r/\gamma_R$ incoherent excitons. Here we have assumed that the reservoir contributes to the nonlinear renormalisation of the exciton frequency in the same way as the strongly-coupled excitons. This is reasonable for an excitonic reservoir at a frequency close to that of the strongly-coupled excitons. If this is not the case then the expression for $g_{\rm eff}$ will differ from that given by a constant multiplier.

Since we deal with CW pumping the field have a harmonic time dependence at frequency $\omega = \omega_e + \delta$ so that we can write their time dependences as $A = A\,(x,z)\exp(-i\delta t)$ and likewise for $\psi$. Substituting these into Eqns. (1) gives a generalised GPE for the photon field in the form Eqn. (2a). Here the linear plus nonlinear (envelope) propagation phase $Q$ and loss $\alpha$ are given in Eqns. (2b) and (2c) respectively and $|\psi|^2$ may be obtained from $|A|^2$ using the real positive valued transcendental equation Eqn. (2d).

$$\left(i\frac{\partial}{\partial z} + \frac{1}{2\beta_e}\frac{\partial^2}{\partial x^2} + Q(|A|^2) + i\alpha(|A|^2)\right)A = 0 \tag{2a}$$

$$Q = \frac{1}{v_g}\left(\delta\left(1 - \frac{|\psi|^2}{|A|^2}\right) + g_{\rm eff}\frac{|\psi|^4}{|A|^2}\right) \tag{2b}$$

$$\alpha = \frac{1}{v_g}\left(\gamma_p + \frac{|\psi|^2}{|A|^2}(\gamma_e + \gamma_r)\right) \tag{2c}$$

$$\left[\left(\delta - g_{\rm eff}\,|\psi|^2\right)^2 + (\gamma_e + \gamma_r)^2\right]|\psi|^2 = \left(\frac{\Omega}{2}\right)^2|A|^2 \tag{2d}$$

$$g_{\rm eff} = g_X\left(1 + \frac{\gamma_r}{\gamma_R}\right) \tag{2e}$$

In fact Eqn. (2d) is cubic in $|\psi|^2$ and, provided $\delta g_{\rm eff} < 0$, has only one real positive (and therefore physical) solution which can be written in closed form, given in Eqns. (3).

$$|\psi|^2 = \sqrt[3]{R + \sqrt{D}} + \sqrt[3]{R - \sqrt{D}} + \frac{2\delta}{g_{\rm eff}} \tag{3a}$$

$$R = -\left(\frac{\delta}{3g_{\rm eff}}\right)^3 + \frac{1}{2}\left(\frac{\Omega}{2g_{\rm eff}}\right)^2|A|^2 - \left(\frac{\delta}{3g_{\rm eff}}\right)\left(\frac{\gamma_e + \gamma_r}{g}\right)^2 \tag{3b}$$

$$D = \left[\frac{1}{2}\left(\frac{\Omega}{2g_{\rm eff}}\right)^2|A|^2\right]^2 - \left(\frac{\Omega}{2g_{\rm eff}}\right)^2\left(\frac{\delta}{3g_{\rm eff}}\right)\left[\left(\frac{\delta}{3g_{\rm eff}}\right)^2 + \left(\frac{\gamma_e + \gamma_r}{g_{\rm eff}}\right)^2\right]|A|^2 + \frac{1}{27}\left(\frac{\gamma_e + \gamma_r}{g_{\rm eff}}\right)^2\left[\left(\frac{\delta}{g_{\rm eff}}\right)^2 + \left(\frac{\gamma_e + \gamma_r}{g_{\rm eff}}\right)^2\right]^2 \tag{3c}$$

The optical field is then described by a function of the transverse coordinate $x$ which evolves with propagation distance $z$ along the waveguide. The intial conditons are fixed at $z = 0$ (where the light enters the waveguide) and the field evolves under the combined action of diffraction and nonlinearity until the result is read out at $z = L$, where $L$ is the spacing between the gratings. The situation is analagous to the temporal evolution of a one dimensional weakly interacting Bose gas governed by a 1D Gross-Pitaevskii equation except in our case the propagation coordinate $z$ plays the role of time. Such systems are expected to have dark soliton solutions.

## S4. Dark Soliton Healing Length and Nonlinearity

The analytical solution for a dark spatial soliton in a nonlinear waveguide is given by Eqn. (4)[10].

$$A = A_0\left[\cos(\phi)\tanh\left(\frac{x - v_s z}{\xi\sqrt{2}}\right) + i\sin(\phi)\right]\exp(-ik_s z) \tag{4}$$

The soliton phase angle $\phi$ and healing length $\xi$ uniquely determine all the properties of the soliton including the transverse velocity $v_s$ and soliton wavenumber $k_s$ via Eqns. (5).

$$v_s = \sin(\phi)\,/\sqrt{\beta L_{\rm NL}} \tag{5a}$$

$$k_s = 1/L_{\rm NL} \tag{5b}$$

Just as in the case of quantised vortices in condensates the healing length is fixed by a balance of the kinetic energy associated with the narrow core and the nonlinear potential energy of the surrounding fluid as quantified in Eqn. (6). Here $L_{\rm NL}$ is the nonlinear length of the background fluid and the waveguide propagation constant $\beta = 23.7\mu m^{-1}$ plays the role of transverse effective

mass. The nonlinear length is related to the density induced energy blueshift of the polariton dispersion $E_{\mathrm{NL}}$ by $L_{\mathrm{NL}} = \hbar v_{\mathrm{g,LP}}/E_{\mathrm{NL}}$ where $v_{\mathrm{g,LP}} = 24$ μm ps$^{-1}$ is the polariton group velocity.

$$\xi = \frac{\sqrt{L_{\mathrm{NL}}}}{\cos(\phi)\sqrt{2\beta}} \tag{6}$$

The healing length is related to the full width at half minimum of the dark intensity notch by FWHM$=2\sqrt{2}\tanh^{-1}\left(\frac{1}{\sqrt{2}}\right)\cdot\xi \approx 2.493\xi$. The size of the phase jump across the soliton is $\pi - 2\phi$. The intensity ratio of the dark notch minimum to the background is given by $\sin^2(\phi)$. Ideal dark solitons may be seeded by any arbitrarily small intensity or phase discontinuity[10]. The phase difference between the fields at $\pm\infty$ must be conserved so that a phase defect in the initial condition generates a single dark soliton with the same phase jump at the core while pure intensity defects generate pairs of solitons with opposite phase[10]. While dark solitons are strictly defined on a background of infinite extent they may also exist on finite backgrounds[15] and in the presence of loss[11]. In this case $\xi$ and $\phi$ evolve adiabatically with $z$ as the background varies. Thus the soliton healing length at a given $z$ depends on the background density at that same position $z$.

Using Eqn. (6) the nonlinear length may be deduced from the soliton core width. This approach is only valid when the transverse field distribution is dominated by the balance of nonlinearity and diffraction rather than purely by diffraction, e.g. the system is in the quasi-solitonic rather than the linear regime. This leads to two conditions which must be fulfilled: (a) The soliton width should be narrower than the notch width in the linear regime and (b) the soliton period $\pi L_{\mathrm{NL}}/2$ should be less than the device length $L$, which gives $\xi < \sqrt{L/(\pi\beta)}$ for the healing length. With the device length of 600μm the FWHM of the notch should therefore be less than 7μm, as well as being less than in the linear regime. One may then obtain the effective polariton-polariton interaction constant using $g = E_{\mathrm{NL}}/n$ where $n$ is the peak density of polaritons. The peak density is related to the power $P(z)$ flowing through a plane at some $z$ using Eqn. (7). Here $w$ is the effective width of the distribution obtained by dividing the integral of the density with $x$ by the peak density.

$$n = \frac{P/(\hbar\omega)}{w \cdot v_{\mathrm{g,LP}}} \tag{7}$$

Combining all the above relations we obtain Eqn. (8) for $g$ in terms of measured parameters.

$$g = \frac{\hbar \cdot w \cdot v_{\mathrm{g,LP}}^2}{2\beta\xi^2\cos^2(\phi)(P/\hbar\omega)} \tag{8}$$

This value is plotted in Fig. 4(b) in the main text for incident powers where the notch width is sufficiently narrow, as discussed above. In the main text we show that the nonlinear parameter deduced from the healing length is consistent with that used in numerical simulations which reproduce the measured intensity distributions as a function of power. This self consistency verifies the validity of the (different) assumptions underlying the two methods.

For reference, the strongly-coupled exciton density per quantum well may be obtained, in the lowest order approximation, using $n_{\mathrm{X}} = n|X|^2/N_{\mathrm{w}}$ where $|X|^2 = 58\%$ is the exciton fraction at the detuning used in this work and $N_{\mathrm{w}}$ is the number of wells. The effective interaction constant (including both reservoir and coherent part) for pure excitons confined in one quantum well is related to the effective lower polariton interaction $g$ according to[21] Eqn. (9).

$$g = \frac{|X|^4}{N_{\mathrm{w}}} g_{\mathrm{eff}} \tag{9}$$

The 'eff' subscript draws attention to the fact that the nonlinearity arises from the reservoir population as well as the coherent exciton field (see section S3). We note that in our system the polarisation is linear so that there are always an equal number of spin up and down polaritons. If one deals with co-circularly polarised excitons, for example in a Bragg microcavity geometry, the constants should be multiplied by a factor of ~2 to account for the fact that the exciton-exciton interaction is known to be anisotropic and much stronger for excitons of the same spin than of opposite spin[21].

## S5. Initial Condition

The initial conditions used in the numerical modelling for the amplitude and phase defects are given by Eqns. (10a) and (10b) respectively. The error functions (or hyperbolic tangent, which has a very similar profile) are included to model the fact that diffractive effects in the free space and optics between the mask and the sample surface smooth out the sharp discontinuities in amplitude and phase introduced at the mask.

$$A_0 = \exp\left(-x^2/w_{\mathrm{b}}^2\right)\cdot \left[1 - a_0\left(\mathrm{erf}\left(\frac{x + w_{\mathrm{n}}/2}{w_{\mathrm{d}}}\right) - \mathrm{erf}\left(\frac{x - w_{\mathrm{n}}/2}{w_{\mathrm{d}}}\right)\right)\right] \tag{10a}$$

$$A_0 = \exp\left(-x^2/w_{\mathrm{b}}^2\right)\cdot \left(\cos(\phi)\tanh\left(\frac{x}{w_{\mathrm{n}}}\right) + i\sin(\phi)\right) \tag{10b}$$

In figure S2 we show the modelled input condition intensity and phase and compare the modelled input and low-power output intensity distributions with those measured experimentally. The modelled output intensity profile was determined using the exact solution of the paraxial waveguide propagation equation in the Fourier domain and using measured experimental parameters for

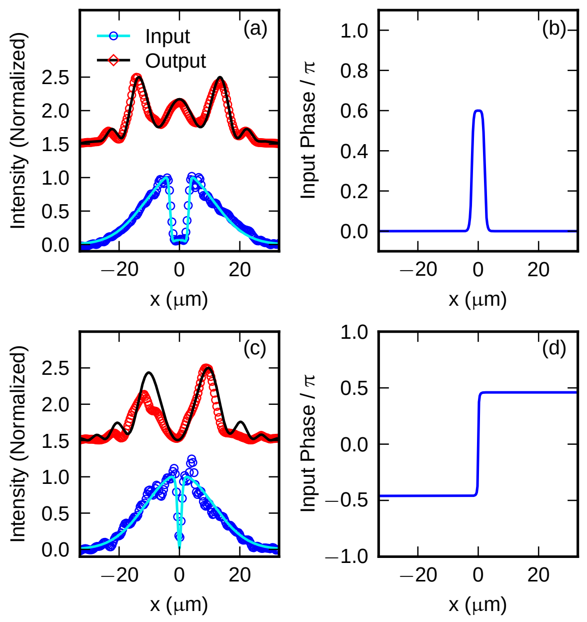


FIG. S2. Comparison of modelled and experimental input and low-power output intensity distributions for amplitude (a) and phase (c) defects. Phase of model initial conditions for amplitude (b) and phase (d) defects.

the waveguide propagation constant and device length. The agreement is very good apart from a discrepancy around $x = -10\,\mu$m in the output field for the phase discontinuity. We attribute this discrepancy to a localised defect in the output grating coupler. The good agreement for both input and output profiles shows that the modelled initial condition amplitude and phase are a close match to the experimental initial condition. We note the non-zero phase and intensity at the position of the dark notch in the case of the amplitude defect. This occurs due to diffraction in the free-space propagation of the laser beam from the mask to the sample surface. These effects are also responsible for the sharp but finite width notch at $x = 0$ in the phase-jump initial condition. For an infinitely sharp phase jump one would not expect to see any notch in the intensity profile. The aforementioned diffraction effects blur the phase jump resulting in the observed finite-width notch in intensity.

* p.m.walker@sheffield.ac.uk


[1] *Exciton Polaritons in Microcavities*, Eds., Timofeev, V. and Sanvitto, D. (Springer, 2014).
[2] P. M. Walker, L. Tinkler, D. V. Skryabin, A. Yulin, B. Royall, I. Farrer, D. A. Ritchie, M. S. Skolnick and D. N. Krizhanovskii *Nature Commun.* **6,** 8317 (2015)
[3] P. M. Walker, L. Tinkler, M. Durska, D. M. Whittaker, I. J. Luxmoore, B. Royall, D. N. Krizhanovskii, M. S. Skolnick, I. Farrer and D. A. Ritchie *Appl. Phys. Lett.* **102,** 012109 (2012)
[4] G. P. Agrawal, *Nonlinear Fibre Optics* (Academic Press, 2001)
[5] M. C. Rechtsman, J. M. Zeuner, Y. Plotnik, Y. Lumer, D. Podolsky, F. Dreisow, S. Nolte, M. Segev, A. Szameit *Nature* **496,** 196-200 (2013)
[6] M. C. Rechtsman, J. M. Zeuner, A. Tünnermann, S. Nolte, M. Segev, A. Szameit *Nature Photon.* **7,** 153-158 (2013)
[7] S. V. Suchkov, A. A. Sukhorukov, J. Huang, S. V. Dmitriev, C. Lee and Y. S. Kivshar. *Laser Photonics Rev.* **10,** 177-213 (2016)
[8] S. Longhi, *Laser Photon Rev.*, **3,** 243-261 (2009)
[9] P. E. Larré and I. Carusotto, *Phys. Rev. A* **92,** 043802 (2015)
[10] Y. S. Kivshar and G. P. Agrawal, *Optical Solitons* (Academic Press, 2003)
[11] Y. S. Kivshar and B. Luther-Davies *Phys. Rep.* **298,** 81-197 (1998)
[12] G. R. Allan, S. R. Skinner, D. R. Andersen and A. L. Smirl, *Opt. Lett.* **16,** 156 (1991)
[13] G. A. Swartzlander, Jr., D. R. Andersen, J. J. Regan, H. Yin and A. E. Kaplan. *Phys. Rev. Lett.* **66,** 1583 (1991)
[14] V. Shandarov, D. Kip, M. Wesner and J. Hukriede, *J. Opt. A: Pure Appl. Opt.* **2,** 500-503 (2000)
[15] Y. S. Kivshar and X. Yang, *Optics Comms.* **107,** 93 (1994)
[16] N. P. Proukakis, N. G. Parker, D. J. Frantzeskakis, and C. S. Adams, *J. Opt. B: Quantum Semiclass. Opt.* **6,** S380-S391 (2004)
[17] D J Frantzeskakis, *J. Phys. A: Math. Theor.* **43,** 213001 (2010)
[18] A. Amo, S. Pigeon, D. Sanvitto, V. G. Sala, R. Hivet, I. Carusotto, F. Pisanello, G. Leménager, R. Houdré, E. Giacobino, C. Ciuti and A. Bramati, *Science* **332,** 1167-1170 (2011)
[19] G. Grosso, G. Nardin, F. Morier-Genoud, Y. Léger and B. Deveaud-Plédran *Phys. Rev. Lett.* **107,** 245301 (2011)
[20] S. Blair and K. Wagner, *Appl. Opt.* **38,** 6749-6772 (1999)
[21] A. S. Brichkin, S. I. Novikov, A. V. Larionov, V. D. Kulakovskii, M. M. Glazov, C. Schneider, S. Höfling, M. Kamp and A. Forchel, *Phys. Rev. B* **84,** 195301 (2011)
[22] S. R. K. Rodriguez, A. Amo, I. Sagnes, L. Le Gratiet, E. Galopin, A. Lemaître, J. Bloch, *Nature Commun.* **7,** 11887 (2016)
[23] M. M. Glazov, H. Ouerdane, L. Pilozzi, G. Malpuech, A. V. Kavokin and A. D'Andrea, *Phys. Rev. B* **80,** 155306 (2009)
[24] M. Vladimirova, S. Cronenberger, D. Scalbert, K. V. Kavokin, A. Miard, A. Lemaître, J. Bloch, D. Solnyshkov, G. Malpuech and A. V. Kavokin, *Phys. Rev. B* **82,** 075301 (2010)
[25] A. V. Sekretenko, S. S. Gavrilov, V. D. Kulakovskii, *Phys. Rev. B* **88,** 195302 (2013)

[26] L. Ferrier, E. Wertz, R. Johne, D. D. Solnyshkov, P. Senellart, I. Sagnes, A. Lemaître, G. Malpuech and J. Bloch, *Phys. Rev. Lett.* **106,** 126401 (2011)
[27] I. Carusotto and C. Ciuti, *Rev. Mod. Phys.* **85,** 299 (2013)
[28] A. Verger, C. Ciuti and I. Carusotto, *Phys. Rev. B* **73,** 193306 (2006)
[29] I. Carusotto, D. Gerace, H. E. Tureci, S. De Liberato, C. Ciuti and A. Imamoğlu. *Phys. Rev. Lett.* **103,** 033601 (2009)
[30] R. O. Umucalılar and I. Carusotto, *Phys. Rev. Lett.* **108,** 206809 (2012)
[31] M. Hafezi, M. D. Lukin and J. M. Taylor, *New Journal of Physics* **15,** 063001 (2013)
[32] X. Chen, Z-C. Gu, Z-X. Liu and X-G. Wen, *Science* **338,** 1604 (2012)
[33] See supplemental section S2 for details of how we determined the coupling efficiency.
[34] P. Cilibrizzi, H. Ohadi, T. Ostatnicky, A. Askitopoulos, W. Langbein, and P. Lagoudakis *Phys. Rev. Lett.* **113,** 103901 (2014)
[35] A. Amo, J. Bloch, A. Bramati, I. Carusotto, C. Ciuti, B. Deveaud, E. Giacobino, G. Grosso, A. Kamchatnov, G. Malpuech, N. Pavloff, S. Pigeon, D. Sanvitto and D. D. Solnyshkov *Phys. Rev. Lett.* **115,** 089401 (2015)
[36] P. Cilibrizzi, H. Ohadi, T. Ostatnicky, A. Askitopoulos, W. Langbein and P. Lagoudakis *Phys. Rev. Lett.* **115,** 089402 (2015)
[37] See supplemental section S1 for more details about the experimental arrangement.
[38] See supplemental section S5 for mathematical expressions for the initial conditions and additional comparison with experiment.
[39] K. Guda, M. Sich, D. Sarkar, P. M. Walker, M. Durska, R. A. Bradley, D. M. Whittaker, M. S. Skolnick, E. A. Cerda-Méndez, P. V. Santos, K. Biermann, R. Hey, D. N. Krizhanovskii. *Phys. Rev. B* **87,** 081309(R) (2013)
[40] See supplemental section S4 for more detailed discussion of soliton properties and a derivation of the relationship between polariton nonlinearity, density and soltion healing length.
[41] D. M. Whittaker, *Phys. Rev. Lett.* **80,** 4791 (1998)
[42] D. N. Krizhanovskii, G. Dasbach, A. A. Dremin, V. D. Kulakovskii, N. A. Gippius, M. Bayer, A. Forschel *Solid State Comms.* **119,** 453-459 (2001)
[43] J. -M. Ménard, C. Poellmann, M. Porer, U. Leierseder, E. Galopin, A. Lemaître, A. Amo, J. Bloch and R. Huber *Nature Commun.* **5,** 4648 (2016)
[44] D. Sarkar, S. S. Gavrilov, M. Sich, J. H. Quilter, R. A. Bradley, N. A. Gippius, K. Guda, V. D. Kulakovskii, M. S. Skolnick and D. N. Krizhanovskii. *Phys. Rev. Lett.* **105,** 216402 (2010)
[45] D. W. Snoke, W. W. Rühle, K. Köhler, K. Ploog *Phys. Rev. B* **55,** 13789 (1997)
[46] J. O. Tollerud, S. T. Cundiff, J. A. Davis *Phys. Rev. Lett.* **117,** 097401 (2016)
[47] See Supplemental Fig. S1(d) for a comparison of experimental and modelled losses.
[48] See supplementl section S3 for details of the derivation of the generalized GPE.
[49] R. Ulrich, *J. Opt. Soc. Am.* **63,** 1419 (1973)
[50] R. Houdré, J. L. Gibernon, P. Pellandini, R. P. Stanley, U. Oesterle, C. Weisbuch, J. O'Gorman, B. Roycroft and M. Ilegems, *Phys. Rev. B.* **52,** 7810 (1995)
